# Supplementary material for: Non-random network connectivity comes in pairs
Source: arXiv:1609.04245 source file (2016-12-13)
Supplement: Supplementary file 1 [file appendix.tex]

\subsection{Two-point distribution}

\subsubsection*{A1}

Solving \eqref{eq:bd1} for $p$ gives
\begin{align}
  p = \frac{\mu-y}{x-y},
\end{align}
which, plugged into \eqref{eq:bd2}, yields
\begin{align}
  \varrho & = \frac{\left(\frac{\mu-y}{x-y}\right)x^2  + \left(1-\frac{\mu-y}{x-y}\right) y^2}{\mu^2} \\ & = \underbrace{\frac{(\mu - y)x^2}{(x-y)\mu^2}}_{\mathrm{(I)}}\,\, + \,\, \underbrace{\frac{y^2}{\mu^2}}_{\mathrm{(II)}}\,\, - \,\, \underbrace{\frac{(\mu - y)y^2}{(x-y) \mu^2}}_{\mathrm{(III)}}.
\end{align}

The summands are
\begin{align}
  \mathrm{(I):} \quad & \frac{(\mu - y)x^2}{(x-y)\mu^2} = \frac{x^2}{(x-y)\mu} - \frac{yx^2}{(x-y)\mu^2} \\
  \mathrm{(II):} \quad &  \frac{y^2}{\mu^2} = \frac{(x-y)y^2}{(x-y)\mu^2} = \frac{xy^2}{(x-y)\mu^2} - \frac{y^3}{(x-y)\mu^2} \\
  \mathrm{(III):} \quad & - \frac{(\mu - y)y^2}{(x-y) \mu^2} = \frac{y^3}{(x-y)\mu^2} - \frac{y^2}{(x-y)\mu}
\end{align}

Putting everything together we get
\begin{align}
  \varrho & =  \frac{x^2 - y^2}{(x-y)\mu} + \frac{xy^2 -yx^2}{(x-y)\mu^2}  = \frac{(x + y) (x-y)}{(x-y)\mu} - \frac{xy (x-y)}{(x-y)\mu^2} \\
  & = \frac{x+y}{\mu} - \frac{xy}{\mu^2}.
\end{align}

\subsubsection*{A2}
Solve \eqref{eq:bd1} for $y$ and since $x \geq \mu$,
\begin{align}
y = \frac{\mu - px}{1-p} \leq \frac{\mu - p\mu}{1-p} = \mu.
\end{align}

%% See aslo: \href{https://www.wolframalpha.com/input/?i=Simplify[%28%28%28c-y%29%2F%28x-y%29%29*x^2%2B%281-%28%28c-y%29%2F%28x-y%29%29%29*y^2%29%2Fc^2]}{Wolfram Alpha}.
